# Supplementary material for: Hierarchically Coherent Multivariate Mixture Networks
Source: arXiv:2305.07089 source file (2023-10-16)
Supplement: Supplementary file 1 [file mixture_ablation.tex]

Throughout our experiments, we observed a \emph{bias-variance trade-off} between the number of mixture components and the CRPS score. When K=1, the CRPS evaluation score is the worst, but improves as we increase the number of mixture components. However, after the number of components surpasses a certain threshold, the CRPS score then begins to deteriorate. We hypothesize that when the mixture has too few components, the model has an insufficient number of parameters to accurately represent the data, causing a worse CRPS score and high bias. If the mixture has too many components, the mode may be over-complicated and over-fitted to the training data, leading to large variance and poor validation performance.

\EDIT{Table CRPS measurements suggest that there is a \emph{bias-variance trade-off} controlled by the Poisson mixture size. When $K=1$, \ours\ model corresponds to Poisson regression and treats each series as probabilistically independent, such model high-bias simple model produced predictions with the worst CRPS. The prediction accuracy improves as the number of Poisson components increases from $K=1$, but the accuracy begins to deteriorate beyond a certain threshold. We hypothesize that a small number of mixture components does not have enough degrees of freedom to describe the data, and too many mixture components lead to over-fitting the training data, resulting in large variance on the validation data.}
% We hypothesize that when $K$ is sufficiently large, the forecast accuracy will reach its optimal point, and when $K$ is further increased, the accuracy will be degraded, \textcolor{red}{possibly due to the non-identifiability of finite Poisson models.}

\EDIT{We observed that the precise value of an optimal Poisson mixture components varies across the datasets. Larger datasets, or datasets with a complex time series correlation structure, appear to benefit from more flexible probability mixtures. \Traffic, our smallest dataset, produced optimal results with $K=25$ components, \TourismL, a medium-sized dataset, produced optimal results with $K=25$ components. Finally \Favorita\, our largest dataset, did not saturate even with the largest number of components we experimented with; we capped the choice of the number of mixture components at $K=100$ due to GPU memory constraints.}

\begin{figure*}[ht]
\centering
\includegraphics[width=0.65\linewidth]{images/CRPSvsComponentsStudy.pdf}
\caption{CRPS score vs Gaussian Mixture Size ablation study. We saw a bias-variance tradeoff corresponding to the number of mixture components for the Labour, Traffic, and TourismLarge datasets. Initially, the CRPS validation score improves as the number of components increases, and reaches an optimal value at K=10 components. From there, we see the CRPS validations score worsens, thus giving us the classic U-shaped tradeoff pattern.} \label{fig:ablation_study_crps_vs_k}
\end{figure*}

\EDIT{Poisson Mixture size ablation study. We found interesting bias-variance trade-offs controlled by the number of mixture components, both \Traffic\ and \TourismL\ have an optimal value of 25 components, beyond which the CRPS validation performance worsens. We observed a classic U-shaped pattern. In the case of \Favorita, the largest dataset, the validation CRPS continued to improve through $K=100$.}
